# Supplementary material for: Moderation Matters:Measuring Conversational Moderation Impact in English as a Second Language Group Discussion
Source: arXiv:2502.18341 source file (2025-02-24)
Supplement: Supplementary file 1 [file PLS_anonymised.pdf]

# Plain Language Statement

School of XXXXXXXXXXXXXXXX/Faculty of XXX

Project: Development of Interactional Competence: Prediction and Quantification on L2 English Dialogue

Responsible Researcher:

Prof XXXXXXXX XXXXXXXX Tel: (XX) XXXX XXXX Email: XXXXXXXX@XXXXXXXX;

Additional Researchers:

Prof XXXXXXXX XXXXXXXX Tel: (XX) XXXX XXXX Email: XXXXXXXX@XXXXXXXX;

Student Researcher:

XXXXXXXX XXXXXXXX Tel: (XX) XXXX XXXX Email: XXXXXXXX@XXXXXXXX;

XXXXXXXX XXXXXXXX Tel: (XX) XXXX XXXX Email: XXXXXXXX@XXXXXXXX;

## Introduction

Thank you for your interest in participating in this research project. The following few pages will provide you with further information about the project, so that you can decide if you would like to take part in this research. Please take the time to read this information carefully. You may ask questions about anything you don't understand or want to know more about. Your participation is voluntary. If you don't wish to take part, you don't have to. If you begin participating, you can also stop at any time.

## What is this research about?

The research is to investigate the discussion and participation patterns of ESL (English as Second Language) speaker in English group discussion. In particular, we are interested in the benefit and effect of the presence of a moderator during the conversation.

What will I be asked to do?

If you agree to participate, you will be asked to provide language samples through group discussion sessions. These sessions may be conducted in a free-style discussion format or be moderated. If applicable, your voice may be recorded. You will be assigned to a group with participants who share similar non-native language backgrounds.

You will take part in one or more discussion sessions, depending on your availability and interest. Each session will include 3 to 5 other participants and will consist of the following:

1. **A themed topic** (e.g., *Modern Romance*).
2. **A set of 3–5 guiding questions** (e.g., *How do dating practices and expectations differ between generations, and what are the main factors driving these differences?*).
3. **A discussion format** that is either **free-flowing** or **moderated**.
4. **A duration of 40–60 minutes** per session.

#### Additional Considerations

- The discussion will be **recorded**, and all data will be **anonymized** before being used for research purposes.
- Some topics may involve **personal or emotional content**. Please consider whether the information you share contains **private details** or could impact your personal life.
- Our research focuses on **language expression and interaction patterns** rather than the authenticity of shared content. You are welcome to remain **anonymous** or modify details when discussing sensitive personal experiences.
- This study primarily involves **text and audio content**, so **turning on your camera is not required**.

What are the possible benefits?

This study on conversational moderation in ESL group discussions offers several potential benefits. It can enhance participants' English proficiency by improving their speaking, listening, and interaction skills in structured discussions. Effective moderation techniques may foster more inclusive and engaging conversations, reducing anxiety and encouraging balanced participation. The findings can contribute to language learning research by identifying best practices for facilitating discussions, which may inform ESL teaching methods and AI-driven moderation tools. Insights from this research may also benefit online learning platforms and multilingual workplaces by optimizing discussion facilitation strategies.

What are the possible risks?

There are few risks associated with this project and these risks are minimal. Potential risks might include research participants finding responding to research tasks difficult or tiring, or feeling shy or anxious about their performance, or worrying about being identified in later reports of the research. Thesis researchers will ensure that participant performance will not affect any of their records beyond the thesis project, such as school records, professional records, etc. Participant data will be used for research purposes only and raw data will only be available to researchers. Participants are assured that their identities will be protected by using pseudonyms (fake names) and removing identifying information.

Do I have to take part?

No. Participation is completely voluntary. You are able to withdraw at any time. You can also withdraw any data that has not been analysed. Participants who withdraw without completing data collection may not receive compensation

Will I hear about the results of this project?

The researcher will provide a summary of finding, or a copy of the completed thesis/paper to participants upon request.

What will happen to information about me?

Data are stored as digital files, e.g., spreadsheets, documents, or audio/video files. It is stored on the student researcher's computer and the University's cloud storage service in password protected files. When analysing the data, participants' names are changed to pseudonyms (fake names) and identifying information is removed, making participants not to be identified. Only the student researcher and the supervisor researcher have access to potentially identifiable data. Data reported in theses and possible later publications is not identifiable. Data is kept by the student researcher for five years after thesis submission or the last publication resulting from the thesis. Where can I get further information?

If you would like more information about the project, please contact the researchers; xxx xxxxx xxxxx@xxxxxx; xxxxx xxxxx xxxxx@xxxxxx or the student researcher in this study: xxx xxx, xxxxxx@xxxxxx.

Who can I contact if I have any concerns about the project?

This project has human research ethics approval from The University of XXXXX. If you have any concerns or complaints about the conduct of this research project, which you do not wish to discuss with the research team, you should contact the XXXXXXXXXX, Office of Research Ethics and Integrity, University of XXXXX, XXXXX. Tel: +XX XXX XXX XXX or Email: XXXXXX@XXXXX All complaints will be treated confidentially. In any correspondence please provide the name of the research team and/or the name or ethics ID number of the research project. Project ID Number: XXXXXX
