# Supplementary material for: Moderation Matters:Measuring Conversational Moderation Impact in English as a Second Language Group Discussion
Source: arXiv:2502.18341 source file (2025-02-24)
Supplement: Supplementary file 2 [file survey.pdf]

# English Second Language Speaker Group Discussion Experience Survey

**Dear Participant,**

Thank you for taking the time to participate in our research study. Your insights and experiences are invaluable to us and will significantly contribute to advancing our understanding of group discussions in second language (SL) learning contexts.

This survey aims to gather your feedback on your experiences during both moderated and un-moderated group discussion sessions. Your responses will help us evaluate the effectiveness of different moderation strategies and improve future SL teaching practices and resources.

The survey should take approximately **3-5 minutes** to complete. All responses are confidential and will be used solely for academic research purposes. Your honest and thoughtful input is greatly appreciated.

If you have any questions or need assistance while completing the survey, please do not hesitate to contact us at [mingbin@unimelb.edu.au](mailto:mingbin@unimelb.edu.au) or [rena.gao@unimelb.edu.au](mailto:rena.gao@unimelb.edu.au).

Thank you again for your valuable contribution to our research.

---

\* Indicates required question

## Personal Information

1. First name \*

---

2. Email

---

3. Which type of sessions have you attended \*

*Mark only one oval.*

- ☐ With moderator
- ☐ Without moderator
- ☐ Both with and without moderator

## 4. Which topics did you attend?

*Check all that apply.*

- ☐ What makes you laugh? What does it convey and how is it perceived?(Laugh)
- ☐ Romantic Relationships in Modern Society (Romance)
- ☐ How to deal with stress? (Stress)
- ☐ How to cope with bosses with different cultural backgrounds (Boss)
- ☐ Understanding Time: Perspectives on How We Perceive, Manage, and Value It (Time)
- ☐ How AI impacts our daily life now and the future?
- ☐ Are you superstitious? Why do people believe in 'weird' things?

How would you rate each of the following statements based on your experience in the **moderated** discussion sessions? (skip if you didn't have any moderated discussion sessions)

Please rate the below statements with the scale of

- 1 (very disagree)
- 2 (somewhat disagree)
- 3 (neither agree or disagree)
- 4 (somewhat agree)
- 5 (very agree)

5. 1. I feel comfortable and encouraged in expressing my opinion and ideas.  
(Comfort Level)

*Mark only one oval.*

|                                                                     |                       |                       |                       |                       |                       |            |
|---------------------------------------------------------------------|-----------------------|-----------------------|-----------------------|-----------------------|-----------------------|------------|
|                                                                     | 1                     | 2                     | 3                     | 4                     | 5                     |            |
| <hr style="border: 0; border-top: 1px solid #ccc; margin: 5px 0;"/> |                       |                       |                       |                       |                       |            |
| Very                                                                | <input type="radio"/> | <input type="radio"/> | <input type="radio"/> | <input type="radio"/> | <input type="radio"/> | Very agree |

6. 2. I feel having the equal opportunity to participate and express my opinions.  
(Participation Opportunities)

*Mark only one oval.*

|                                                                     |                       |                       |                       |                       |                       |            |
|---------------------------------------------------------------------|-----------------------|-----------------------|-----------------------|-----------------------|-----------------------|------------|
|                                                                     | 1                     | 2                     | 3                     | 4                     | 5                     |            |
| <hr style="border: 0; border-top: 1px solid #ccc; margin: 5px 0;"/> |                       |                       |                       |                       |                       |            |
| Very                                                                | <input type="radio"/> | <input type="radio"/> | <input type="radio"/> | <input type="radio"/> | <input type="radio"/> | Very agree |

7. 3. I feel have been listened, understood and respected by others in the discussion.

(Mutual respect)

*Mark only one oval.*

|      |                       |                       |                       |                       |                       |            |
|------|-----------------------|-----------------------|-----------------------|-----------------------|-----------------------|------------|
|      | 1                     | 2                     | 3                     | 4                     | 5                     |            |
| Very | <input type="radio"/> | <input type="radio"/> | <input type="radio"/> | <input type="radio"/> | <input type="radio"/> | Very agree |

8. 4. I feel I can understand clearly other's opinions.  
(Communication Ease)

*Mark only one oval.*

|      |                       |                       |                       |                       |                       |            |
|------|-----------------------|-----------------------|-----------------------|-----------------------|-----------------------|------------|
|      | 1                     | 2                     | 3                     | 4                     | 5                     |            |
| Very | <input type="radio"/> | <input type="radio"/> | <input type="radio"/> | <input type="radio"/> | <input type="radio"/> | Very agree |

9. 5. I feel the conversation content were productive and insightful. (Discussion Quality)

*Mark only one oval.*

|      |                       |                       |                       |                       |                       |            |
|------|-----------------------|-----------------------|-----------------------|-----------------------|-----------------------|------------|
|      | 1                     | 2                     | 3                     | 4                     | 5                     |            |
| Very | <input type="radio"/> | <input type="radio"/> | <input type="radio"/> | <input type="radio"/> | <input type="radio"/> | Very agree |

10. 6. I feel the conversation was engaging and interactive. (Interactive Engagement)

*Mark only one oval.*

|      |                       |                       |                       |                       |                       |            |
|------|-----------------------|-----------------------|-----------------------|-----------------------|-----------------------|------------|
|      | 1                     | 2                     | 3                     | 4                     | 5                     |            |
| Very | <input type="radio"/> | <input type="radio"/> | <input type="radio"/> | <input type="radio"/> | <input type="radio"/> | Very agree |

11. 7. I found the session useful for improving oral English.  
(Learning Outcomes)

*Mark only one oval.*

|      |                       |                       |                       |                       |                       |            |
|------|-----------------------|-----------------------|-----------------------|-----------------------|-----------------------|------------|
|      | 1                     | 2                     | 3                     | 4                     | 5                     |            |
| Very | <input type="radio"/> | <input type="radio"/> | <input type="radio"/> | <input type="radio"/> | <input type="radio"/> | Very agree |

12. 8. I feel more confident in speaking English in front of multiple strangers.  
(Learning Outcomes)

*Mark only one oval.*

|      |                       |                       |                       |                       |                       |            |
|------|-----------------------|-----------------------|-----------------------|-----------------------|-----------------------|------------|
|      | 1                     | 2                     | 3                     | 4                     | 5                     |            |
| Very | <input type="radio"/> | <input type="radio"/> | <input type="radio"/> | <input type="radio"/> | <input type="radio"/> | Very agree |

13. 9. I was satisfied and enjoyed with the overall experience of the conversation.  
(Overall)

*Mark only one oval.*

|      |                       |                       |                       |                       |                       |            |
|------|-----------------------|-----------------------|-----------------------|-----------------------|-----------------------|------------|
|      | 1                     | 2                     | 3                     | 4                     | 5                     |            |
| Very | <input type="radio"/> | <input type="radio"/> | <input type="radio"/> | <input type="radio"/> | <input type="radio"/> | Very agree |

How would you rate each of the following statements based on your experience in the **non-moderated** discussion sessions? (skip if you didn't have any **non-moderated** discussion sessions)

Please rate the below statements with the scale of 1 (very disagree), 2(somewhat disagree), 3(neither agree or disagree), 4 (somewhat agree), 5 (very agree).

14. 1. I feel comfortable and encouraged in expressing my opinion and ideas.  
(Comfort Level)

*Mark only one oval.*

|      |                       |                       |                       |                       |                       |            |
|------|-----------------------|-----------------------|-----------------------|-----------------------|-----------------------|------------|
|      | 1                     | 2                     | 3                     | 4                     | 5                     |            |
| Very | <input type="radio"/> | <input type="radio"/> | <input type="radio"/> | <input type="radio"/> | <input type="radio"/> | Very agree |

15. 2. I feel having the equal opportunity to participate and express my opinions.  
(Participation Opportunities)

*Mark only one oval.*

|      |                       |                       |                       |                       |                       |            |
|------|-----------------------|-----------------------|-----------------------|-----------------------|-----------------------|------------|
|      | 1                     | 2                     | 3                     | 4                     | 5                     |            |
| Very | <input type="radio"/> | <input type="radio"/> | <input type="radio"/> | <input type="radio"/> | <input type="radio"/> | Very agree |

16. 3. I feel have been listened, understood and respected by others in the discussion.  
(Mutual respect)

*Mark only one oval.*

|      |                       |                       |                       |                       |                       |            |
|------|-----------------------|-----------------------|-----------------------|-----------------------|-----------------------|------------|
|      | 1                     | 2                     | 3                     | 4                     | 5                     |            |
| Very | <input type="radio"/> | <input type="radio"/> | <input type="radio"/> | <input type="radio"/> | <input type="radio"/> | Very agree |

17. 4. I feel I can understand clearly other's opinions.  
(Communication Ease)

*Mark only one oval.*

|      |                       |                       |                       |                       |                       |            |
|------|-----------------------|-----------------------|-----------------------|-----------------------|-----------------------|------------|
|      | 1                     | 2                     | 3                     | 4                     | 5                     |            |
| Very | <input type="radio"/> | <input type="radio"/> | <input type="radio"/> | <input type="radio"/> | <input type="radio"/> | Very agree |

18. 5. I feel the conversation content were productive and insightful. (Discussion Quality)

*Mark only one oval.*

|      |                       |                       |                       |                       |                       |            |
|------|-----------------------|-----------------------|-----------------------|-----------------------|-----------------------|------------|
|      | 1                     | 2                     | 3                     | 4                     | 5                     |            |
| Very | <input type="radio"/> | <input type="radio"/> | <input type="radio"/> | <input type="radio"/> | <input type="radio"/> | Very agree |

19. 6. I feel the conversation was engaging and interactive. (Interactive Engagement)

*Mark only one oval.*

|      |                       |                       |                       |                       |                       |            |
|------|-----------------------|-----------------------|-----------------------|-----------------------|-----------------------|------------|
|      | 1                     | 2                     | 3                     | 4                     | 5                     |            |
| Very | <input type="radio"/> | <input type="radio"/> | <input type="radio"/> | <input type="radio"/> | <input type="radio"/> | Very agree |

20. 7. I found the session useful for improving oral English. (Learning Outcomes)

*Mark only one oval.*

|      |                       |                       |                       |                       |                       |            |
|------|-----------------------|-----------------------|-----------------------|-----------------------|-----------------------|------------|
|      | 1                     | 2                     | 3                     | 4                     | 5                     |            |
| Very | <input type="radio"/> | <input type="radio"/> | <input type="radio"/> | <input type="radio"/> | <input type="radio"/> | Very agree |

21. 8. I feel more confident in speaking English in front of multiple strangers. (Learning Outcomes)

*Mark only one oval.*

|      |                       |                       |                       |                       |                       |            |
|------|-----------------------|-----------------------|-----------------------|-----------------------|-----------------------|------------|
|      | 1                     | 2                     | 3                     | 4                     | 5                     |            |
| Very | <input type="radio"/> | <input type="radio"/> | <input type="radio"/> | <input type="radio"/> | <input type="radio"/> | Very agree |

22. 9. I was satisfied and enjoyed with the overall experience of the conversation.  
(Overall)

*Mark only one oval.*

|      |                       |                       |                       |                       |                       |            |
|------|-----------------------|-----------------------|-----------------------|-----------------------|-----------------------|------------|
|      | 1                     | 2                     | 3                     | 4                     | 5                     |            |
| Very | <input type="radio"/> | <input type="radio"/> | <input type="radio"/> | <input type="radio"/> | <input type="radio"/> | Very agree |

### Final section

23. If you have attended both the moderated and non-moderated sessions, which type of discussion would you prefer?

*Mark only one oval.*

- ☐ I prefer moderated discussion
- ☐ I prefer non-moderated free discussion
- ☐ I have no preference either type of discussions.
- ☐ I only participated one type of discussion, so can't compare.

24. What benefits did you perceive from attending the session?

*Check all that apply.*

- ☐ Deepening my understanding of the topic through group discussion.
- ☐ Practicing English speaking (skills, vocabulary etc.) and communication skills.
- ☐ Improving how I convey and articulate my ideas during discussions.
- ☐ Improving public speaking/speaking with a group of people.
- ☐ Getting to know others better through in-depth conversations.
- ☐ Other: \_\_\_\_\_
